# Supplementary material for: Rethinking Metadynamics: from bias potentials to probability distributions
Source: arXiv:1909.07250 ancillary file (2020-02-14)
Supplement: Supplementary file 1 [file OPES-SI.pdf]

# SUPPORTING INFORMATION
# Rethinking Metadynamics: from bias potentials to probability distributions

Michele Invernizzi and Michele Parrinello*

E-mail: parrinello@phys.chem.ethz.ch

## Algorithmic details

### Kernel density compression

As discussed in the main text, it is impractical to describe the probabilities as a sums of all the Gaussians deposited. In metadynamics (MetaD) and in adaptive umbrella sampling this difficulty is usually circumvented by mapping the bias on an auxiliary grid. Here we shall reduce the number of Gaussians needed to represent the probability by using a kernel compression algorithm borrowed from signal processing literature.[1] This algorithm has been previously used only for post-processing estimation, and never with a shrinking bandwidth, but it turned out to be especially convenient in our setup, thanks to the recursive nature of our method.

We restrict ourselves to the consideration of Gaussian kernels with diagonal bandwidths, the generalisation to more complex kernels being straightforward. Thus, as in the main text, we write:

$$G(\mathbf{s},\mathbf{s}') = h e^{-\frac{1}{2}\sum_i \left(\frac{s_i - s'_i}{\sigma_i}\right)^2} . \tag{1}$$

To measure of the distance between a point $\mathbf{s}'$ and a kernel $G$ we consider the Mahalanobis distance, that in our case reads:

$$d(\mathbf{s}', G) = \sqrt{\sum_i \left(\frac{s_i - s'_i}{\sigma_i}\right)^2} . \tag{2}$$

Let us suppose that we have to deposit the $n$-th kernel $G(\mathbf{s},\mathbf{s}^{(n)})$ at position $\mathbf{s}^{(n)}$, after the ones previously deposited have been compressed to $N$ kernels $G_k$, where in general as $n$ grows we expect $N \ll n$. The algorithm then goes as follows:

1. find the minimun distance between the new point and the compressed kernels, $d_{\min} = \min_k d(\mathbf{s}^{(n)}, G_k)$
2. check if this distance is smaller than a given threshold, $d_t$:
   a. if $d_{\min} < d_t$ merge the new kernel $G(\mathbf{s},\mathbf{s}^{(n)})$ with the closest one $G_{k_{\min}}$. Then go back to step 1, using instead of $\mathbf{s}^{(n)}$ the new center of the merged kernel
   b. if $d_{\min} \geq d_t$ add the new kernel $G(\mathbf{s},\mathbf{s}^{(n)})$ to the compressed ones

When merging two Gaussians $G_1$ and $G_2$ the new Gaussian $G(\mathbf{s},\mathbf{s}')$ will have the following parameters:

$$h = h_1 + h_2 \tag{3}$$
$$\mathbf{s}' = h^{-1}(h_1\mathbf{s}_1 + h_2\mathbf{s}_2) \tag{4}$$
$$\boldsymbol{\sigma}^2 = h^{-1}[h_1(\boldsymbol{\sigma}_1^2 + \mathbf{s}_1^2) + h_2(\boldsymbol{\sigma}_2^2 + \mathbf{s}_2^2)] - \mathbf{s}'^2 \tag{5}$$

This simple merging rule applies only to Gaussians with diagonal bandwidth, however is possible to extend it also to the general case.[1]

We found that $d_t = 1$ is a good default value. However sometimes it might be useful to adopt a higher threshold, in order to reduce the total

number of kernels, at the cost of obtaining a coarser estimate of the probability density.

This compression algorithm differs from that of Ref. 1 mostly for the addition of the recursive rule at the end of 2.a. We found this step very useful especially when the CVs dimensionality is greater than one, because without it the minimum distance between the deposited kernels quickly becomes smaller than $d_t$, and the total number of kernels may grow much faster. This extra step does add an overhead to the algorithm, so in our implementation we also provide the option not to perform it.

The total number of compressed kernels will always grow in time, but it soon reaches a sort of plateau, with minimal growth. It is in general not easy to guess a priori how many kernels will be needed, since it depends not only on the dimensionality of the CV space, but also on the features of the free energy surface and on the range of exploration. However, in our experience the total number of kernels is always reasonable, and generally much smaller than the number of points in a typical grid of the same dimensionality.

The overall computational cost of the biasing scheme scales roughly linearly with the total number of compressed kernels, since at each time step we need to sum over all them in order to estimate the bias and the forces due to the bias. A way of greatly reduce the computational cost would be to implement a neighbor list scheme, but at this point this has been left to future development.

This bias representation has some advantages when compared to the grid representation more commonly used, in particular:

- the user does not need to guess in advance the CV region that will be explored, kernels will be deposited only where necessary
- it can handle a higher dimensional CV space, while grids typically already struggle at three/four dimensions
- it allows changing the scale used for the description of the bias, a feature that we found very useful

## Bandwidth rescaling

The kernels bandwidth is rescaled according to Eq. 6 of the main text:

$$\sigma_i^{(n)} = \sigma_i^{(0)} [N_{\text{eff}}^{(n)} (d+2)/4]^{-1/(d+4)} \,, \qquad (6)$$

where the effective sample size at $n$-th step is:

$$N_{\text{eff}}^{(n)} = \frac{\left(\sum_k^n w_k\right)^2}{\sum_k^n w_k^2} \,. \qquad (7)$$

We find useful to define $w_0 = 1$, so that at the beginning of the simulation $N_{\text{eff}}^{(0)} = 1$. This choice makes the estimate of the effective sample size more robust, especially at the very fist steps of the simulation.

We notice that the fact that the bandwidth is rescaled, requires that also the height of the deposited Gaussian is adjusted accordingly, since

$$h = \prod_i \frac{1}{\sigma_i \sqrt{2\pi}} \,. \qquad (8)$$

## Normalization factor

According to its definition, in Eq. 5 of the main text, the probability estimator $\tilde{P}(\mathbf{s})$ is normalized to 1 over a boundless CV space. By adding the normalization factor $Z_n$, defined as in Eq. 7 of the main text, we take into account for the actually explored CV space, $\Omega_n$. To calculate $Z_n$ we take advantage of our compressed kernel representation, and consider the centers of the kernels as points for a Monte Carlo integration:

$$Z_n = \frac{1}{N} \sum_k^N \tilde{P}(\mathbf{s_k}) = \frac{1}{NS} \sum_{k,k'}^N G(\mathbf{s_k}, \mathbf{s_{k'}}) \,, \qquad (9)$$

where $G(\mathbf{s_k}, \mathbf{s_{k'}})$ are the compressed Gaussians, $N$ is their total number, and $S = \sum_k^n w_k$ is the global normalization of the KDE. $Z_n$ changes accordingly to the explored space $\Omega_n$, and typically converges as soon as no new CV space region is explored. The above normalization factor also helps correcting the possible changes in the global normalization $S$ due to the compression algorithm.

The estimate in Eq. 9 scales quadratically with the number of compressed kernels $N$. In

our implementation however, we avoid this by calculating only the changes with respect to the previous value, $Z_n = Z_{n-1} + \Delta Z_n$, which instead scales linearly in $N$.

## The barrier parameter

In the current implementation of the method, there is a parameter called barrier, that should be roughly equal to the free energy barrier $\Delta E$ that the bias should help overcome. We use this value to set the bias factor $\gamma = \beta \Delta E$ and the regularization parameter $\epsilon = e^{-\beta\Delta E/(1-1/\gamma)}$.

According to Eq. 8 of the main text, the minimum value that the bias can assume is reached when $\tilde{P}(\mathbf{s}) = 0$, and with the given choice of $\epsilon$ we have:

$$\min_{\mathbf{s}} V_n(\mathbf{s}) = -\Delta E \tag{10}$$

The maximum value of the bias is instead less easy to obtain, because changes according to the normalization factor $Z_n$. However it is typically only few $k_B T$, so that in practice the maximum deposited bias, $\Delta V_{\max}$, is not too much higher than $\Delta E$.

It is in principle possible to set a hard limit to $\Delta V_{\max}$, e.g. by adaptively adjust the $\epsilon$ value, but we prefer to have some tolerance with respect to the provided estimate of the barrier $\Delta E$, since it is generally not easy to guess it correctly before running simulations.

We chose to link the bias factor $\gamma$ to the value of the barrier $\Delta E$ because $\gamma$ is not a crucial parameter for the convergence speed, as it is the case for MetaD. However it is also possible to set the value of $\gamma$ independently, in order to fine tune the shape of the target distribution. This can be useful e.g. in case a high dimensional CV space, where one typically wants to restrict as much as possible the explored space to speed up sampling.

# Results on model systems

We implemented our method in a development version of the PLUMED[2] plugin, and we plan to add it to the official PLUMED code. All the code and the input files needed to reproduce the following results are openly available in the Materials Cloud Archive (www.materialscloud.org), as `materialscloud:2019.0063`, and on the PLUMED-NEST[3] (www.plumed-nest.org), as `plumID:19.068`.

## Suboptimal double well

We first test our new method on the simple toy model, first presented in Ref. 4, that consists in a particle moving on a 2D potential $U(x, y)$ with Langevin dynamics, see Fig. 2 of main text. The potential is a rotated Wolfe-Quapp, the temperature of the Langevin dynamics is $T = \beta = 1$ and the friction coefficient is 10.

We want to model a double well system with a suboptimal CV, thus we bias only $x$. In this simple system we can directly calculate the free energy profile along $x$ by numerical integration on a grid:

$$F(x) = -\frac{1}{\beta} \log \int_{-3}^{3} e^{-\beta U(x,y)} dy \,, \tag{11}$$

and also the free energy difference $\Delta F$, that we define as follows:

$$\Delta F = -\frac{1}{\beta} \log \frac{\int_0^3 e^{-\beta F(x)} dx}{\int_{-3}^0 e^{-\beta F(x)} dx} \,. \tag{12}$$

We run simulations with both OPES and MetaD, using input parameters as similar as possible. In particular the bias factor $\gamma = 10$, the deposition stride is 500 time steps and the initial bandwidth is $\sigma = 0.185815$ (equal to the unbiased standard deviation in the minimum). Using the reference from Eq. 11 we also run simulations with a static bias $V(x) = -(1 - 1/\gamma)F(x)$, that is the bias that both OPES and MetaD reach at convergence. The MetaD simulations use Gaussians with initial height $h = 1$ and deposit bias only in the interval $[-2.9, 2.9]$, to avoid pushing the system out of the $[-3, 3]$ range in which the potential is defined. This last precaution is not needed for the OPES and the static bias simulations.

In order to compare the different methods we select 100 initial conditions from an unbiased run in which the system remained in the deeper

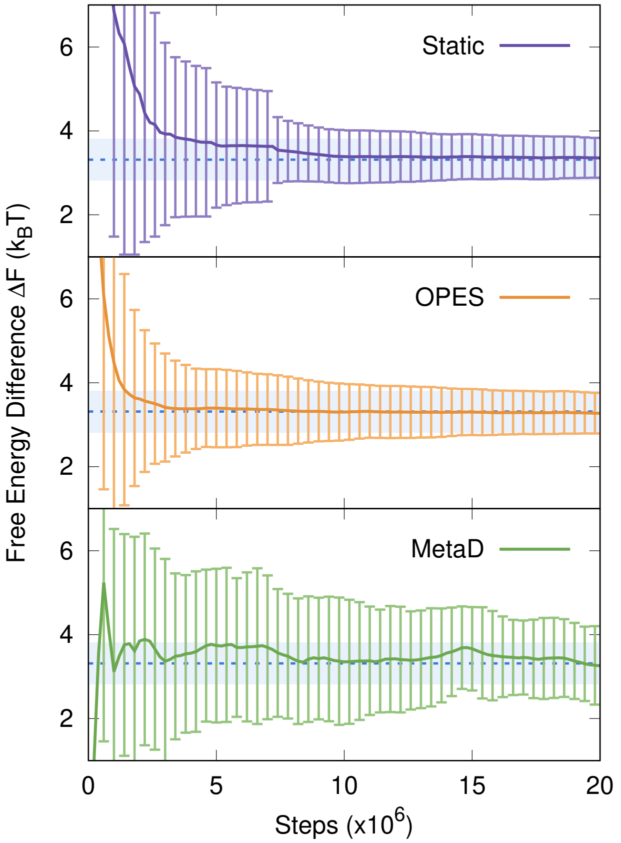


Figure 1: The free energy difference of the double well model, calculated with different methods. For the static bias case the reweight estimate is shown, while for the others the estimate obtained from the applied bias. Average and standard deviation over 100 independent runs are shown.

basin. These configurations are used to start 100 independent runs for each of the methods investigated. The free energy difference $\Delta F$ is calculated from the free energy estimator given by $F_n(x) = -(1-1/\gamma)^{-1}V_n(x)$, except for the static bias case where reweighting (Eq. 1 of main text) is used. Fig. 1 shows the average $\Delta F$ obtained, together with the standard deviation, as a function of time.

It is interesting to notice that OPES yields the best estimate, outperforming also the reference run with a perfect static bias. This is due to the fact that all the 100 replicas start form the same basin (thus $\Delta F_n = 0$ at the beginning), and a dynamic bias allows for a faster first transition than a static one, thus more quickly correcting this wrong initial estimate.

The number of compressed kernels that build the probability estimate is always smaller than 80, for all of the OPES simulations.

**Reweighting.** It is also possible to obtain an estimate of the free energy and $\Delta F$ via reweighting, instead of using the one obtained from the bias potential. To perform reweighting we follow Eq. 1 of main text, using as probability estimator a weighted KDE. In order to reweight a non-static bias one usually must discard the initial non-adiabatic part of the trajectory, where the bias changes too fast. Unfortunately it is not always clear how much one should cut out. For this reason we find it useful to invert the trajectory and plot the reweighted estimate as a function of time, as in Fig. 2. The plot shows all the possible choices for initial truncation, with on the abscissa axis the amount of steps truncated. At the far left is the estimate obtained without discarding any point, at half of the plot is the reweighting obtained only from the second half of the trajectory and so on. Thus the final part of the trajectory is always used, which makes sense, since it is the most close to convergence.

There are different ways of reweighting MetaD. Since we do know the real $F(x)$ of our toy model, we can use the real $c(t)$, instead of one of its estimates.[5,6] At step $n$ the "real"

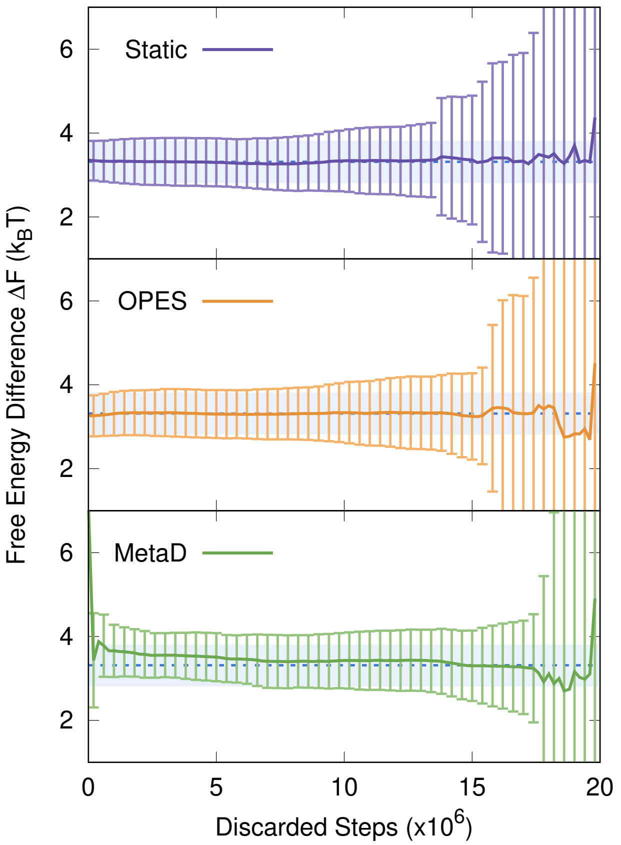


Figure 2: The $\Delta F$ of the double well model from the same simulations used for Fig. 1, but obtained through reweighting. The trajectory has been time-inverted before reweighing, in order to show all the possible initial truncations (see explanation in the text). The MetaD reweighting is obtained using a perfect $c(t)$, obtained using the real $F(x)$.

$c(t)$ is obtained via a grid integration:

$$c_n = -\frac{1}{\beta}\log\frac{\int_{-3}^{3} e^{-\beta[F(x)+V_n(x)]}dx}{\int_{-3}^{3} e^{-\beta F(x)}dx} \,. \qquad (13)$$

This provides a better reweighting, because it removes the noise from the $c(t)$ estimation.

By looking at Fig. 2 we can see that, as expected, in the static bias case there is no need to cut any initial transient. In OPES the reweighting estimate is not significantly influenced by keeping the initial part of the simulation, even though it is non-adiabatic, and it gives an estimated $\Delta F$ very similar to the one actually used during the biasing. In MetaD instead the reweighing estimate has a smaller standard deviation compared to the direct estimate, but one should discard a significant part of the trajectory in order to obtain a correct estimate.

**Sampling efficiency: well-tempered vs uniform.** Using this toy model we can also quantify the gain in sampling efficiency provided by using a well-tempered target instead of a uniform one. To do so, we look at the effective sample size $N_{\text{eff}} = (\sum_k w_k)^2 / \sum_k w_k^2$ which provides an estimate of the efficiency of the importance sampling we are doing. We run as before with 100 different initial conditions, using a well-tempered static bias $V(x) = -(1-1/\gamma)F(x)$ with $(\gamma = 10)$ and a uniform one $V(x) = -F(x)$. For the well-tempered case we obtain $N_{\text{eff}}/N = 0.0236 \pm 0.042$ while for the uniform $N_{\text{eff}}/N = 0.0117 \pm 0.022$. This means that given the same number of steps $N$, using a well-tempered target in this case provides roughly twice the effective sample size compared to a uniform target, and thus any quantity estimated from it will have a smaller statistical uncertainty.

## Alanine dipeptide

For the alanine dipeptide simulations we use GROMACS[7] patched with PLUMED. The setup is the same of Ref. 4, namely: canonical (NVT) simulation in a vacuum, Amber99-SB[8] force field, time step 0.002 fs, temperature 300 K, and velocity rescaling thermostat.[9]

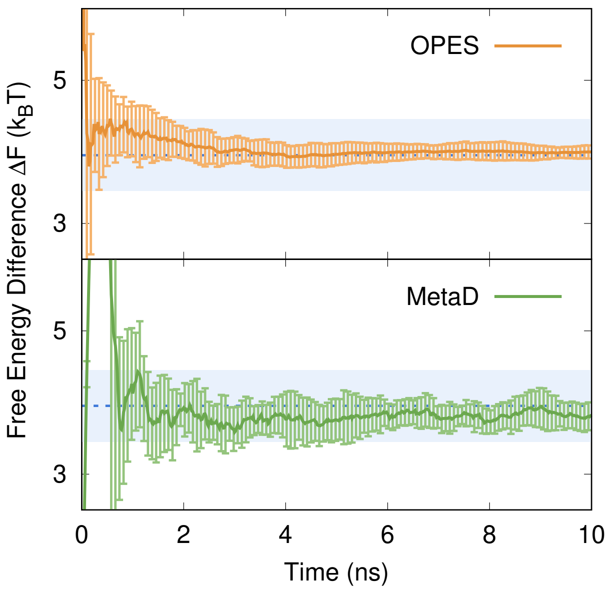


Figure 3: The free energy difference for alanine dipeptide, calculated with different methods. The estimate is obtained form the applied bias, average and standard deviation over 10 independent simulations are shown.

We run OPES and MetaD, using the same bias factor $\gamma = 10$ and deposition stride of 500 time steps. For MetaD we used the typical standard parameters for alanine dipeptide, namely $\sigma_\phi = \sigma_\psi = 0.35$ rad, and Gaussian height $h = 1.2$ kJ/mol. For the OPES simulations we choose an initial bandwidth $\sigma_\phi = \sigma_\psi = 0.15$ rad, which is roughly the smaller of the standard deviations one gets by running a short unbiased simulation in the two basins, and a barrier parameter $\Delta E = 50$ kJ/mol. Such $\Delta E$ value would lead to a default bias factor $\gamma \approx 20$, but we set it instead to $\gamma = 10$, in order to facilitate the comparison with MetaD. We run 10 independent simulations for each method, starting from initial configurations taken from a long unbiased run in the most stable basin (basin A). Fig. 3 shows the average and the standard deviation of the free energy difference $\Delta F$, for each method. We define the free energy difference in units of $k_BT$ as:

$$\Delta F = -\log \frac{\int_A e^{-\beta F(\phi,\psi)} d\phi\, d\psi}{\int_B e^{-\beta F(\phi,\psi)} d\phi\, d\psi}, \qquad (14)$$

where $A = \{\phi \in [0, 2.3], \psi \in [-\pi, \pi]\}$ and $B$ is the complementary region in the CVs space.

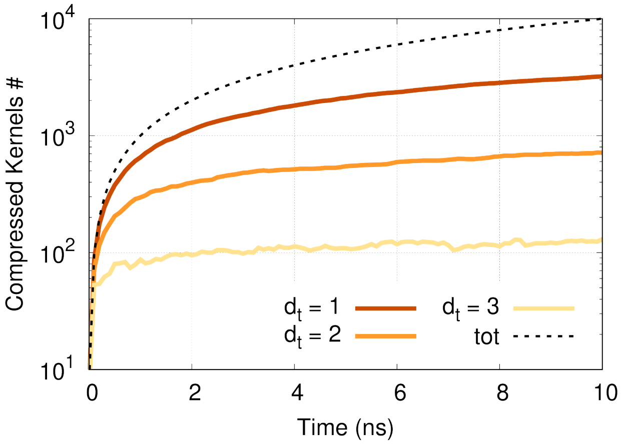


Figure 4: The typical number of compressed kernels used in the alanine dipeptide simulations. The black dotted line shows the total number of deposited kernels. After 100 ns with compression threshold $d_t = 1$ about 68% of the deposited kernels have been merged, while with $d_t = 3$ about 99%. In this $d_t = 3$ case the bias is very coarse, but still allows for good sampling and the reweighting estimate of $\Delta F$ falls within 1 $k_BT$.

The number of kernels used in the OPES simulations for representing the probability distribution, and thus the bias, is shown in Fig. 4. In this case we also test some other values of the compression threshold $d_t$, but all the results shown in other figures and in the main text are obtained with $d_t = 1$. For the MetaD simulations of alanine dipeptide we use a 100x100 grid with spline interpolation.

## Alanine tetrapeptide

With the same computational setup of alanine dipeptide, we simulate alanine tetrapeptide, which has 3 $\phi$ and 3 $\psi$ angles, see Fig. 5. Using the 3 $\phi$ angles as CVs would be enough to get a good sampling, but in order to test the performance in higher dimensions we run simulations with 6 CVs, using all the angles.

Fig. 6 shows the trajectories of the 6 dihedral angles for OPES and MetaD. It can be seen how OPES provides an extremely fast exploration also in such high dimensional case. In principle one could decide to fix the OPES bias after a

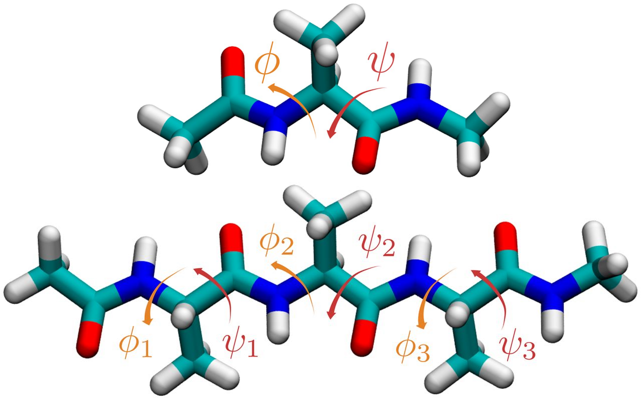


Figure 5: The alanine dipeptide and alanine tetrapeptide molecules, with their Ramachandran angles.

few nanoseconds, and use it as static bias to perform umbrella sampling, in the spirit of Ref.s 10,11.

We notice that the performance of MetaD can be improved by tweaking the parameters, e.g. using a bigger initial height for the Gaussians, but we could not find any combination of parameters giving an exploration qualitatively similar to OPES. Using parallel bias metadynamics[12] (PBMetaD) brings much better performances in such high CV space. From the point of view of the exploration however it was still less efficient that OPES, requiring a few nanoseconds to find all the basins (but we only tested with the standard parameters, without any tweaking). It would be interesting to implement in OPES the same target distribution that PBMetaD reaches at convergence, because it covers a much smaller CV volume than well-tempered, while still sampling all the relevant basins. Having a smaller CV volume to sample can help a lot in converging, especially when a big number of CVs is employed.

In Fig. 7 a free energy estimate obtained form reweighting the previous shown OPES simulation is shown, compared with a reference one obtained from a much longer simulation performed with only the 3 $\phi$ angles. We chose to show the free energy projected onto the $\phi_2$-$\phi_3$ space, because these are the two angles harder to sample. It is remarkable that after only 1 nanosecond (1000 kernels deposited) all the metastable basins have been sampled, and the free energy already shows all the relevant features.

# References

(1) Sodkomkham, D.; Ciliberti, D.; Wilson, M. A.; Fukui, K.-I.; Moriyama, K.; Numao, M.; Kloosterman, F. Kernel density compression for real-time Bayesian encoding/decoding of unsorted hippocampal spikes. *Knowledge-Based Systems* **2016**, *94*, 1–12.

(2) Tribello, G. A.; Bonomi, M.; Branduardi, D.; Camilloni, C.; Bussi, G. PLUMED 2: New feathers for an old bird. *Computer Physics Communications* **2014**, *185*, 604–613.

(3) The PLUMED consortium, Promoting transparency and reproducibility in enhanced molecular simulations. *Nature Methods* **2019**, *16*, 670–673.

(4) Invernizzi, M.; Parrinello, M. Making the Best of a Bad Situation: A Multiscale Approach to Free Energy Calculation. *Journal of Chemical Theory and Computation* **2019**, *15*, 2187–2194.

(5) Tiwary, P.; Parrinello, M. A time-independent free energy estimator for metadynamics. *Journal of Physical Chemistry B* **2015**, *119*, 736–742.

(6) Giberti, F.; Cheng, B.; Tribello, G. A.; Ceriotti, M. Iterative unbiasing of quasi-equilibrium sampling. **2019**,

(7) Abraham, M. J.; Murtola, T.; Schulz, R.; Páll, S.; Smith, J. C.; Hess, B.; Lindahl, E. GROMACS: High performance molecular simulations through multi-level parallelism from laptops to supercomputers. *SoftwareX* **2015**, *1-2*, 19–25.

(8) Hornak, V.; Abel, R.; Okur, A.; Strockbine, B.; Roitberg, A.; Simmerling, C. Comparison of multiple Amber force fields and development of improved protein

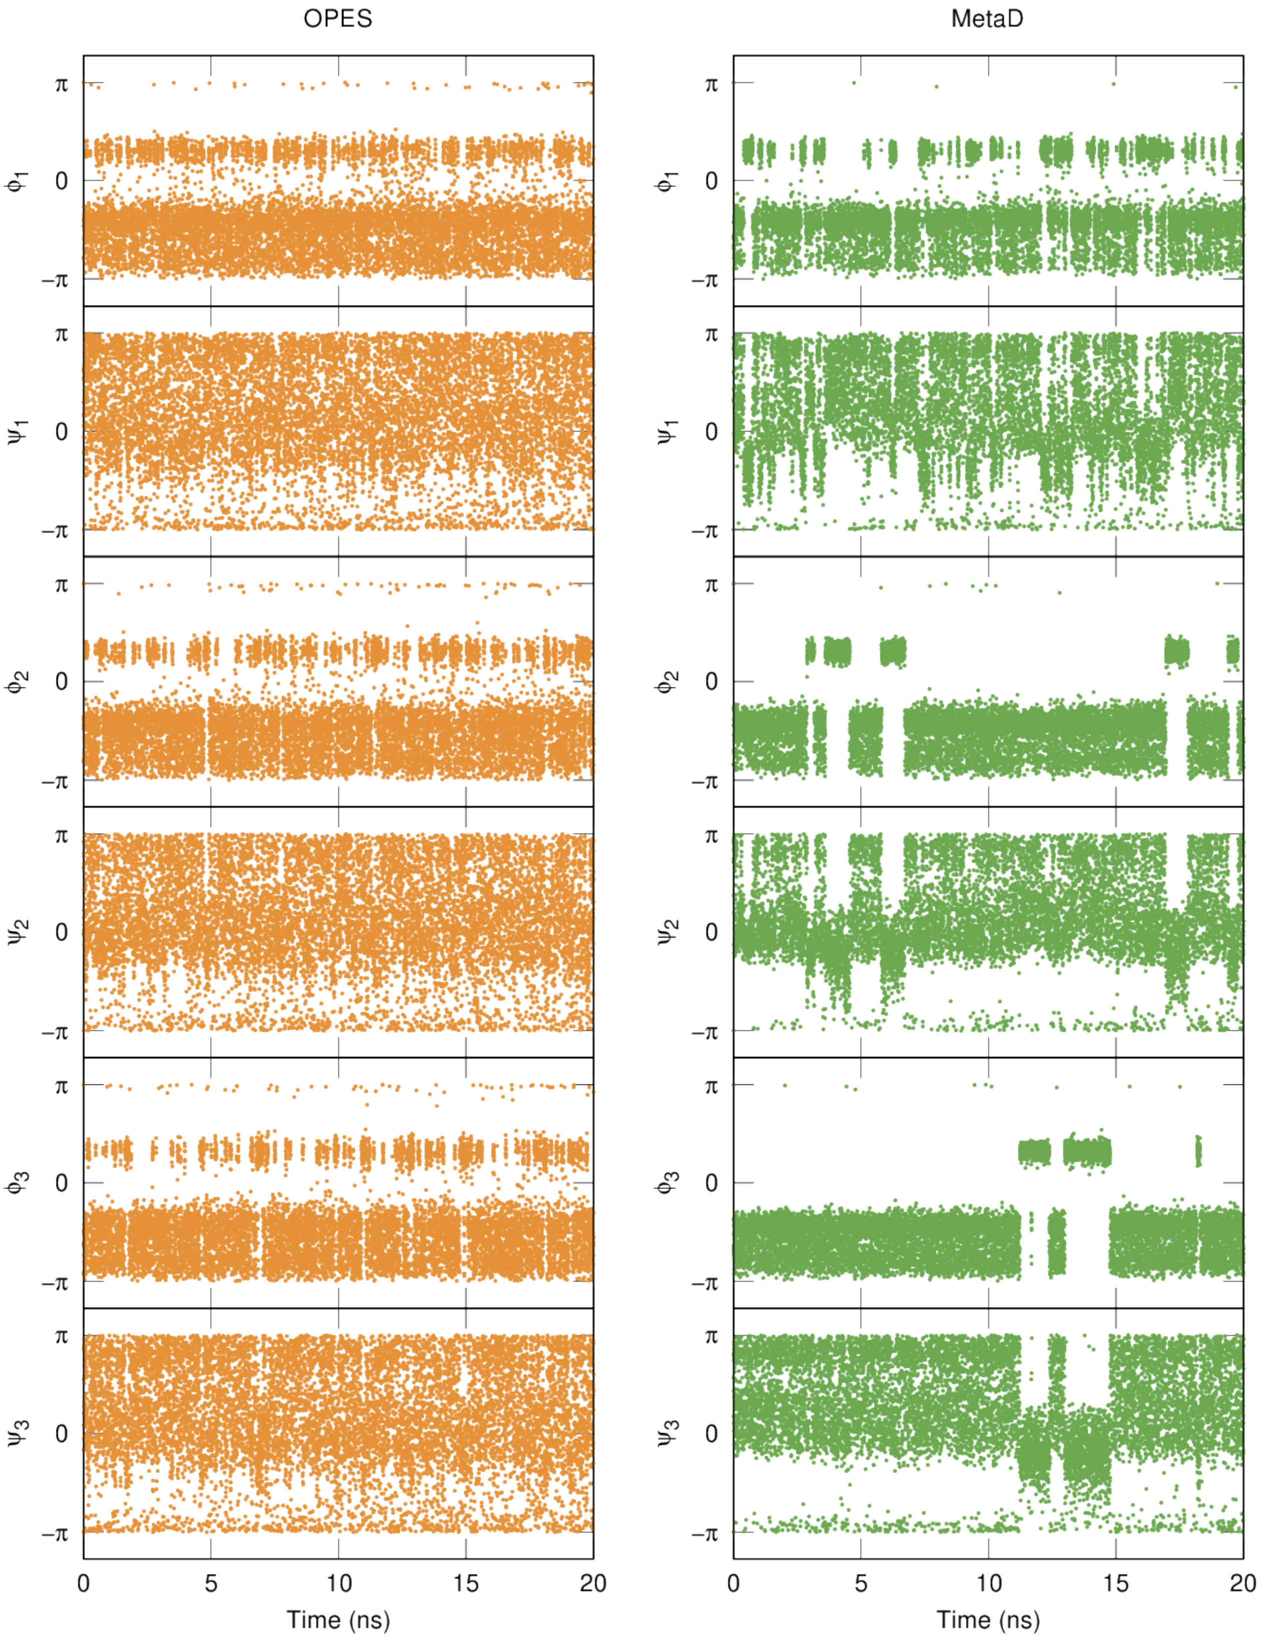


Figure 6: The trajectory of the 6 dihedral angles of alanine tetrapeptide, obtained by biasing all of them with OPES and MetaD respectively.

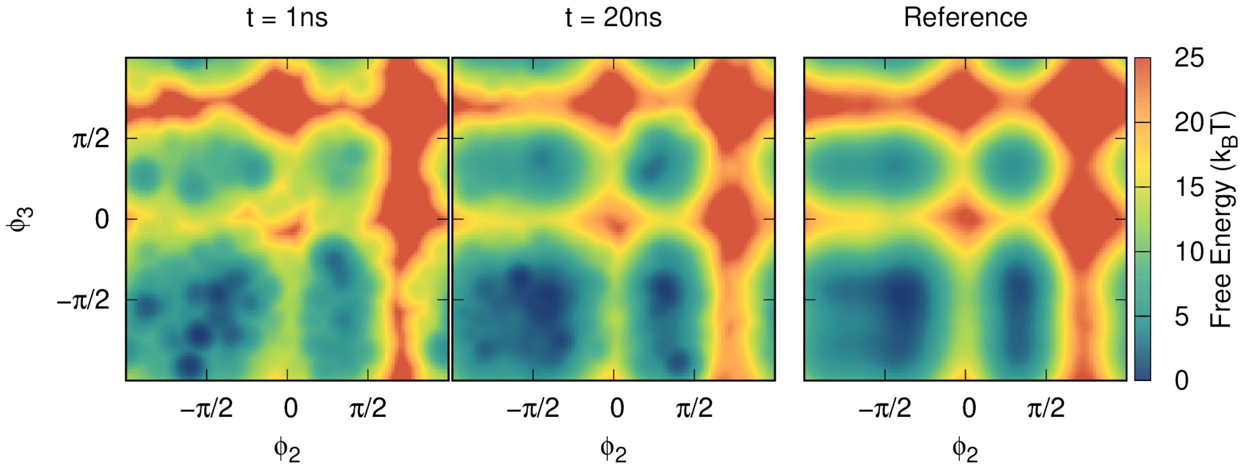


Figure 7: Free energy for alanine tetrapeptide, obtained by reweighting over the $\phi_2, \phi_3$ plane the OPES simulation shown in Fig. 6. The reference free energy comes from a 100ns OPES simulation performed using only the three $\phi$ angles as CVs.

backbone parameters. *Proteins: Structure, Function, and Bioinformatics* **2006**, *65*, 712–725.

(9) Bussi, G.; Donadio, D.; Parrinello, M. Canonical sampling through velocity rescaling. *The Journal of Chemical Physics* **2007**, *126*, 014101.

(10) Invernizzi, M.; Valsson, O.; Parrinello, M. Coarse graining from variationally enhanced sampling applied to the Ginzburg–Landau model. *Proceedings of the National Academy of Sciences* **2017**, *114*, 3370–3374.

(11) Bonati, L.; Zhang, Y.-Y.; Parrinello, M. Neural networks-based variationally enhanced sampling. *Proceedings of the National Academy of Sciences* **2019**, 201907975.

(12) Pfaendtner, J.; Bonomi, M. Efficient Sampling of High-Dimensional Free-Energy Landscapes with Parallel Bias Metadynamics. *Journal of Chemical Theory and Computation* **2015**, *11*, 5062–5067.
